# Supplementary material for: Adjusting the Ground Truth Annotations for Connectivity-Based Learning to Delineate
Source: arXiv:2112.02781 source file (2022-12-24)
Supplement: Supplementary file 1 [file appendix.tex]

\section{Appendix 1}
It is important for the functioning of our algorithm that the values of $D$ are (sub-)differentiable with respect to the ground truth deformation parameters $\phi$.
To clarify this, we provide a more formal definition of the value of $D$ at voxel in position $q$:  
\begin{equation} \label{eq:d1}
D^q_i\big(y^\star_i(\phi_i)\big)=\min\{\delta(y^\star_i(\phi_i),q),d\} \;,
\end{equation}
where $\delta(y^\star_i(\phi_i),q)$ denotes the distance between the voxel $q$ and the closest point on the annotation $y^\star_i$, computed as  
\begin{equation} \label{eq:d2}
\delta\big(y^\star_i(\phi_i),q\big)=\min_{(u,v) \in E_i} \min_{0\le \alpha \le 1}|\alpha (p^u_i+\phi^u_i)+(1-\alpha) (p^v_i+\phi^v_i)-q|_2 \;,
\end{equation}
where the minimization over $\alpha$ serves to find the point on edge $(u,v)$, that is closest to $q$.
We can see that the distance~\eqref{eq:d2} is differentiable with respect to $\phi$, except for the pixels which are equidistant to two different edges of the annotation, and for which the outer minimum is not unique.
However, for these pixels, the function is sub-differentiable, and still allows for backpropagation of gradients.

The sub-gradients are ...
\begin{equation}
aaa
\end{equation}

\section{Appendix 2}

Various possible loss-distance field combinations...
